# Supplementary material for: VideoMV: Consistent Multi-View Generation Based on Large Video Generative Model
Source: arXiv:2403.12010 source file (2024-03-18)
Supplement: Supplementary file 4 [file supp_mm_train.tex]

\section{Multi-domain Generation}
Applying VideoMV to multi-domain generation is easy. We show the training process of our multi-domain multi-view generation using the cross-domain attention module in Wonder3D~\cite{Long2023Wonder3DSI}. As depicted in \cref{fig:supp_rgbnd}, multi-domain data are aligned coherently, which is especially beneficial for downstream 3D reconstruction pipelines as demonstrated in \cite{Long2023Wonder3DSI}. In the future, we will focus on how to recover better geometry and texture based on the dense multi-view images generated by VideoMV.

\begin{figure}[htbp]
% \vspace{-1.0em}
  \centering
  \includegraphics[width=1.0\linewidth]{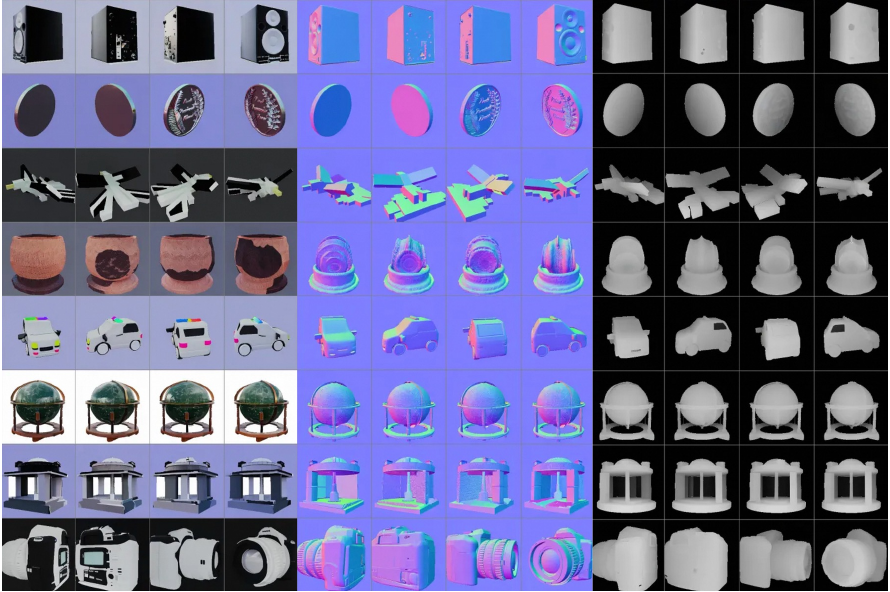}
  \caption{Visual results of the training process of multi-modal generation.}
  \label{fig:supp_rgbnd}
% \vspace{-2.0em}
\end{figure}

% \section{}
